# Supplementary material for: A Machine Learning System for Retaining Patients in HIV Care
Source: arXiv:2006.04944 source file (2020-06-01)
Supplement: Supplementary file 1 [file appendix.tex]

\section{Temporal Cross Validation}

Figure 1 Temporal Cross Validation on EMR Dataset Using temporal cross validation results in the 11 sets of model building (red) and validation datasets (blue). The solid lines indicate the time periods of the appointments included in the model building or validation datasets. The dotted lines represent the lag in time needed to calculate the outcome e.g., for a prediction made for an appointment on Feb 1, 2009, we need to consider the time period of Feb 1, 2009 - Aug 1, 2009 in order to compute the outcome of failure to access care in 6 months. For the outcome of failure to be retained in care, this lag is for 12 months, i.e. from Feb 1, 2009 – Feb 1, 2010. This lag is needed to ensure that no data that is used for validation is included in the model building. At any point in time, we use the maximum available data for model building. Models are then selected using the performance across all the validation data sets

\section{Features Used}
\todo{maybe???}
